# Supplementary material for: When Coordination Is Avoidable: A Monotonicity Analysis of Organizational Tasks
Source: arXiv:2602.18673 source file (2026-07-25)
Supplement: Supplementary file 1 [file pnas-si.pdf]

# Supporting Information for When Coordination Is Avoidable: A Monotonicity Analysis of Organizational Tasks

Harang Ju  
Carey Business School, Johns Hopkins University

## Contents

|          |                                                   |            |
|----------|---------------------------------------------------|------------|
| <b>1</b> | <b>SI Text S1. Formal Preliminaries</b>           | <b>S2</b>  |
| 1.1      | CALM in Multi-Agent Terms . . . . .               | S2         |
| 1.2      | Thompson’s Interdependence (Formalized) . . . . . | S2         |
| <b>2</b> | <b>SI Text S2. Proofs</b>                         | <b>S3</b>  |
| 2.1      | Bridge Theorem Proofs . . . . .                   | S3         |
| 2.2      | Feedback Boundary Proofs . . . . .                | S4         |
| <b>3</b> | <b>SI Text S3. Heuristic Classification Tests</b> | <b>S4</b>  |
| <b>4</b> | <b>SI Text S4. Extended Related Work</b>          | <b>S4</b>  |
| 4.1      | Organizational Theory . . . . .                   | S4         |
| 4.2      | Malone-Crowston Dependency Mapping . . . . .      | S6         |
| <b>5</b> | <b>SI Text S5. Full APQC Corpus</b>               | <b>S6</b>  |
| <b>6</b> | <b>SI Text S6. O*NET Full Results</b>             | <b>S8</b>  |
| <b>7</b> | <b>SI Text S7. LLM Classifier Validation</b>      | <b>S8</b>  |
| <b>8</b> | <b>SI Text S8. Simulation Protocol</b>            | <b>S9</b>  |
| <b>9</b> | <b>SI Text S9. Sensitivity Analysis</b>           | <b>S10</b> |
| 9.1      | Reclassification Range . . . . .                  | S10        |
| 9.2      | Decomposition Dependence . . . . .                | S10        |
| 9.3      | Hidden Constraints . . . . .                      | S11        |

# 1 SI Text S1. Formal Preliminaries

This section states the formal definitions underlying the execution model and Thompson’s interdependence types in two steps. We first restate the CALM execution model in multi-agent terms, replacing distributed nodes with agents. We then formalize Thompson’s three interdependence categories in that same apparatus.

## 1.1 CALM in Multi-Agent Terms

The following definitions recast the CALM framework [1, 2] using agents rather than distributed nodes.

**Definition S1** (Multi-agent task execution). *A multi-agent task execution is a tuple  $(\mathcal{A}, E, \rightarrow, \text{Obs})$  where  $\mathcal{A} = \{a_1, \dots, a_n\}$  is a finite set of agents;  $E$  is a set of events;  $\rightarrow$  is the happened-before partial order on  $E$  [3]; and  $\text{Obs} : \mathcal{H} \rightarrow \mathcal{P}(\mathcal{O})$  maps each history to a set of admissible observable outcomes, where  $\mathcal{H}$  is the set of all histories of  $(E, \rightarrow)$  and  $\mathcal{O}$  is the set of all possible outcomes.*

A history  $H$  is a downward-closed subset of  $(E, \rightarrow)$ : if  $e \in H$  and  $e' \rightarrow e$ , then  $e' \in H$ .

**Definition S2** (History extension).  *$H_1$  is a prefix of  $H_2$ , written  $H_1 \sqsubseteq H_2$ , if  $H_1 \subseteq H_2$  and  $H_1$  is downward-closed in  $(H_2, \rightarrow)$ .*

**Definition S3** (Outcome order). *An outcome order  $\preceq$  is a partial order on  $\mathcal{O}$  that captures when one outcome refines another. The order is task-specific. For tasks whose outputs are sets of results, the natural order is set inclusion:  $o_1 \preceq o_2$  iff  $o_1 \subseteq o_2$ . For tasks whose outputs are tuples (e.g., resource allocations), the natural order is component-wise:  $(x_1, \dots, x_n) \preceq (y_1, \dots, y_n)$  iff  $x_i \leq y_i$  for all  $i$ .*

**Definition S4** (Coordination-free implementation). *An implementation is coordination-free if (i) it only exposes correct outcomes and (ii) it permits all causally admissible histories: no agent is ever blocked to prevent future inconsistency [1, 2].*

**Definition S5** (Monotone and non-monotone specifications). *A task specification (the pair  $(\text{Obs}, \preceq)$  from a given execution) is monotone if for all histories  $H_1 \sqsubseteq H_2$  and all outcomes  $o \in \text{Obs}(H_1)$ , there exists  $o' \in \text{Obs}(H_2)$  with  $o \preceq o'$ . It is non-monotone if there exist  $H_1 \sqsubseteq H_2$  and  $o \in \text{Obs}(H_1)$  such that no  $o' \in \text{Obs}(H_2)$  satisfies  $o \preceq o'$ .*

By the CALM Coordination Theorem, a task specification admits a coordination-free implementation if and only if it is monotone [1, 2, 4].

## 1.2 Thompson’s Interdependence (Formalized)

Thompson’s three categories each impose distinct structural constraints on the agent dependency graph and the task’s output space. A functional programming analogy sharpens the intuition. Pooled tasks compose like pure functions (independent, freely parallelizable, no shared state). Sequential tasks thread output through a monotone pipeline (ordered, no backflow). Reciprocal tasks demand mutable shared state (read-write conflicts, synchronization required). The underlying distinction is the same in both taxonomies. Outputs that only accumulate can be merged freely; outputs that can retract require coordination to remain consistent.

**Definition S6** (Pooled interdependence). *A task has pooled interdependence if: (1) it decomposes into sub-tasks  $T_1, \dots, T_n$  assignable to agents  $a_1, \dots, a_n$ ; (2) all cross-agent event pairs are concurrent (no causal dependencies); (3) each sub-task specification is monotone; and (4) the output space  $(\mathcal{O}, \preceq)$  is a join-semilattice, and the aggregate outcome is the join  $\mu(o_1, \dots, o_n) = o_1 \sqcup \dots \sqcup o_n$ . This is the algebraic structure underlying CRDTs [5].*

**Definition S7** (Sequential interdependence). *A task has sequential interdependence if: (1) agents are ordered  $a_{\pi(1)}, \dots, a_{\pi(n)}$  with causal dependencies from  $a_{\pi(k)}$  to  $a_{\pi(k+1)}$ ; (2) the dependency is unidirectional (DAG); and (3) each agent's local output function  $f_k$  is non-retractive (order-preserving):  $o \preceq o' \implies f_k(o) \preceq f_k(o')$ .*

**Definition S8** (Reciprocal interdependence). *A task has reciprocal interdependence if: (1) the agent dependency graph contains a cycle (bidirectional causal dependency); and (2) the mutual dependency is constraining: at least one agent's admissible outcomes shrink as a function of the other's actions.*

## 2 SI Text S2. Proofs

### 2.1 Bridge Theorem Proofs

The following proofs verify that the structural conditions in Definitions S6–S8 compose to yield the claimed monotonicity properties.

*Proof of Theorem 1(a): Pooled  $\implies$  Monotone.* Let  $H \sqsubseteq H'$  be histories. Decompose by agent:  $H = H^1 \cup \dots \cup H^n$ , and likewise  $H' = (H')^1 \cup \dots \cup (H')^n$ . Since cross-agent events are concurrent (condition 2),  $H^i \sqsubseteq (H')^i$  for each agent  $i$ . Sub-task monotonicity (condition 3) ensures each agent's output refines under history extension. The join-semilattice property (condition 4) then guarantees  $o_1 \sqcup \dots \sqcup o_n \preceq o'_1 \sqcup \dots \sqcup o'_n$ , so the aggregate is monotone.  $\square$

*Proof of Theorem 1(b): Sequential  $\implies$  Monotone under Causal Ordering.* The composition of non-retractive functions is non-retractive: if  $o \preceq o'$ , then  $f_1(o) \preceq f_1(o')$ , hence  $f_2(f_1(o)) \preceq f_2(f_1(o'))$ , and so on. Causal delivery ensures each pipeline stage processes refined input. The specification is monotone over causally ordered histories.  $\square$

*Proof of Theorem 1(c): Reciprocal  $\implies$  Non-Monotone.* Let  $T$  be a task with reciprocal interdependence. By Definition S8, the dependency graph contains a cycle, so there exist agents  $a_i$  and  $a_j$  with bidirectional causal dependency, and the mutual dependency is constraining: at least one agent's admissible outcomes shrink as a function of the other's actions. Without loss of generality, suppose  $a_j$ 's actions constrain  $a_i$ . Let  $H_1$  be a history in which  $a_i$  has acted but  $a_j$  has not yet acted within the cycle. Because  $a_j$  has not yet constrained  $a_i$ , there exists some  $o \in \text{Obs}(H_1)$  reflecting  $a_i$ 's unconstrained output. Now let  $H_2 = H_1 \cup \{e_j\}$ , where  $e_j$  is an action by  $a_j$  in the causal cycle. Because the dependency is constraining,  $a_i$ 's admissible outcomes shrink, so  $o$  is no longer valid. Any outcome  $o' \in \text{Obs}(H_2)$  must respect the tighter constraint, and because the constraint shrinks the admissible set rather than extending it, no such  $o'$  satisfies  $o \preceq o'$ . This is exactly the condition for a non-monotone specification (Definition S5). (As an illustration, consider agents sharing a budget  $B = 100$  with invariant  $\text{spend}_1 + \text{spend}_2 \leq B$  and component-wise outcome order. If  $a_1$  proposes  $\text{spend}_1 = 70$ , then  $(70, 30) \in \text{Obs}(H_1)$ . When  $a_2$  proposes  $\text{spend}_2 = 50$ , the pair  $(70, 50)$  violates the invariant, and no refinement of  $(70, 30)$  is consistent with both proposals.)  $\square$

## 2.2 Feedback Boundary Proofs

*Proof of Proposition 2(a).* Let  $H_1 \sqsubseteq H_2$  where  $H_2$  includes feedback message  $m$  from  $a_j$  to  $a_i$ . Since feedback is additive, the upstream agent incorporates  $m$  without retracting prior output, so  $a_i$ 's updated output satisfies  $o_i \preceq o'_i$ . Since downstream functions are non-retractive, the refinement propagates. The specification remains monotone.  $\square$

*Proof of Proposition 2(b).* Retractive feedback produces  $o''_i$  with  $o_i \not\preceq o''_i$ , so  $o \in \text{Obs}(H_1)$  may have no refinement in  $\text{Obs}(H_2)$ , violating monotonicity. The causal cycle with constraining dependency satisfies Definition S8 (reciprocal interdependence).  $\square$

## 3 SI Text S3. Heuristic Classification Tests

The Bridge Theorem requires classifying a task's interdependence structure, which in turn requires reasoning about dependency graphs and output spaces. For practitioners who need a quick classification without formal verification, Table S1 distills the theorem into five plain-language tests. Each test operationalizes a sufficient condition for non-monotonicity identified in Theorem 1. Tests 1–4 screen for non-monotonicity; Test 5 confirms monotonicity. The tests are conservative by design, with errors falling toward over-coordination rather than under-coordination.

Table S1: Five plain-language heuristic tests for monotonicity classification at runtime. Tests 1–4 screen for non-monotonicity; Test 5 confirms monotonicity.

| Step | Test                   | Question                                                         | If YES    | If NO     |
|------|------------------------|------------------------------------------------------------------|-----------|-----------|
| 1    | Shared Finite Resource | Do sub-tasks draw from a shared pool?                            | Non-mono. | Continue  |
| 2    | Negation               | Do constraints require ensuring absence?                         | Non-mono. | Continue  |
| 3    | Retraction             | Can one agent's output make another's logically incorrect?       | Non-mono. | Continue  |
| 4    | Dependency             | Does correctness depend on specific content of another's output? | Non-mono. | Continue  |
| 5    | Merge                  | Can all outputs always be combined validly?                      | Monotonic | Non-mono. |

## 4 SI Text S4. Extended Related Work

### 4.1 Organizational Theory

Several traditions in organizational theory address when and why coordination is needed. We trace how the Bridge Theorem provides a formal criterion that cuts across these frameworks.

Organizations are information-processing systems, and the structure of a task determines how much processing capacity its execution requires. Galbraith [6] argued that greater task uncertainty demands greater organizational capacity, either by reducing the need for information (through slack resources and self-contained tasks) or by increasing it (through vertical information systems and lateral relations). The Bridge Theorem identifies the formal boundary within this framework.

Table S2: Worked examples applying the heuristic tests to six representative tasks.

| # | Task                                              | Triggering test      | Class     | Thompson   |
|---|---------------------------------------------------|----------------------|-----------|------------|
| 1 | Market analysis across 5 regions                  | Merge: YES           | Mono.     | Pooled     |
| 2 | Cross-functional hiring: 3 teams, 10 candidates   | Shared Resource: YES | Non-mono. | Reciprocal |
| 3 | R&D budget: 4 divisions, \$2M                     | Shared Resource: YES | Non-mono. | Reciprocal |
| 4 | Quarterly planning: depts. write objectives       | Merge: YES           | Mono.     | Pooled     |
| 5 | Multi-chapter style guide: consistent terminology | Dependency: YES      | Non-mono. | Reciprocal |
| 6 | Sequential report: sec. 3 builds on sec. 2        | Dependency: YES      | Non-mono. | Sequential |

Monotonic tasks have inherently low information-processing requirements because new information never invalidates prior work. Non-monotonic tasks require the additional capacity that coordination provides.

The monotonicity boundary also governs which coordination mechanisms organizations deploy. Mintzberg [7] catalogued five mechanisms ranging from mutual adjustment through direct supervision to three forms of standardization (of work processes, outputs, and skills), with organizations reserving the costliest for the most unpredictable work. Mutual adjustment parallels Thompson’s reciprocal interdependence, mapping through the Bridge Theorem to non-monotonic tasks that provably require coordination. Standardization governs routine work, the organizational analog of monotonic tasks where outputs accumulate without conflict.

A related structural insight is that complex systems are nearly decomposable. Simon [8] argued that effective organizations consist of semi-independent modules with strong internal and weak external coupling. Monotonic tasks formalize this weak coupling, because modules can operate independently when their outputs never conflict. Colfer and Baldwin [9] extend the modularity argument in their survey of the “mirroring hypothesis,” finding that organizational structure mirrors technical architecture most strongly when interdependence is high. The Bridge Theorem explains the asymmetry. Reciprocal (non-monotonic) tasks demand tight coupling between organizational and technical boundaries, while pooled and sequential (monotonic) tasks do not.

The framework also sharpens the economic analysis of coordination. Coase [10] argued that firms exist to reduce the transaction costs of market coordination, and Williamson [11] formalized this into transaction cost economics, where governance structures minimize these costs. Before asking how to minimize coordination costs, however, one should ask whether coordination is needed at all. Coordination overhead on monotonic tasks buys nothing, the organizational analog of paying for insurance on events that cannot occur. Ouchi [12] extended this reasoning to the choice among markets, bureaucracies, and clans, arguing that the right governance form depends on output measurability and goal alignment. The Bridge Theorem narrows the scope of that choice, because if a task is monotonic, coordination is unnecessary regardless of the governance form, and the decision among Ouchi’s three mechanisms applies only to the non-monotonic fraction of the task portfolio.

Finally, the framework connects to group performance and AI. Steiner’s [13] process loss model decomposes group performance as  $\text{Actual} = \text{Potential} - \text{Process Losses}$ . The Coordination Tax formalizes which losses are structurally unnecessary, distinguishing overhead that buys correctness from overhead that does not. More recently, Lee and Makridis [14] developed a model characterizing how AI affects the coordination demands of individual work activities. Their analysis complements ours in that we span both individual (O\*NET) and team-level (APQC) tasks and provide a formal

criterion for when coordination is necessary rather than merely costly.

## 4.2 Malone-Crowston Dependency Mapping

The organizational frameworks above describe coordination qualitatively. A more direct formal link exists through the Malone-Crowston dependency taxonomy [15], which classifies inter-task dependencies into four types.

| Dependency type   | Thompson mapping | CALM classification | Coordination need |
|-------------------|------------------|---------------------|-------------------|
| Task-subtask      | Pooled           | Monotone            | None              |
| Producer-consumer | Sequential       | Monotone (causal)   | Ordering only     |
| Shared resources  | Reciprocal       | Non-monotone        | Full coordination |
| Simultaneity      | Reciprocal       | Non-monotone        | Full coordination |

**I-Confluence.** A related formalization from the database literature captures the same intuition from the consistency perspective. Given system invariants  $\mathcal{I}$  and agent operations  $\{o_1, \dots, o_n\}$ , the operations are I-confluent with respect to  $\mathcal{I}$  if, for any two agents executing independently from valid states, merging their states always satisfies  $\mathcal{I}$  [2, 16]. Tasks with shared-resource or simultaneity dependencies fail I-confluence for the same reason they are non-monotone, because independent execution can produce states that violate global invariants.

## 5 SI Text S5. Full APQC Corpus

Table S3 lists all 65 APQC tasks with their Thompson interdependence type and CALM monotonicity label. Tasks are grouped by APQC category and classified at Level-2/3 granularity (team-level workflows with 2–5 agents).

Table S3: Full 65-task corpus with APQC categories, Thompson classifications, and CALM monotonicity labels. Tasks are classified at APQC Level-2/3 granularity.

| #  | APQC Category       | Task                                           | Thompson   | CALM |
|----|---------------------|------------------------------------------------|------------|------|
| 5  | Vision & Strategy   | Allocate strategic investment budget           | Reciprocal | NM   |
| 3  | Vision & Strategy   | Assess organizational capabilities             | Pooled     | M    |
| 2  | Vision & Strategy   | Conduct competitive landscape analysis         | Pooled     | M    |
| 4  | Vision & Strategy   | Develop and cascade KPIs from strategy         | Sequential | M-O  |
| 1  | Vision & Strategy   | Develop strategic plan components              | Pooled     | M    |
| 6  | Products & Services | Conduct market requirements research           | Pooled     | M    |
| 7  | Products & Services | Design product feature specifications          | Pooled     | M    |
| 8  | Products & Services | Evaluate vendor proposals for components       | Pooled     | M    |
| 10 | Products & Services | Prioritize product backlog with fixed capacity | Reciprocal | NM   |
| 9  | Products & Services | Stage-gate product development review          | Sequential | M-O  |
| 15 | Marketing & Sales   | Allocate marketing campaign budget             | Reciprocal | NM   |
| 12 | Marketing & Sales   | Analyze regional sales performance             | Pooled     | M    |
| 13 | Marketing & Sales   | Conduct customer segmentation analysis         | Pooled     | M    |
| 11 | Marketing & Sales   | Develop multi-channel marketing content        | Pooled     | M    |

| #  | APQC Category            | Task                                                         | Thompson   | CALM |
|----|--------------------------|--------------------------------------------------------------|------------|------|
| 14 | Marketing & Sales        | Qualify and route inbound leads                              | Sequential | M-O  |
| 20 | Physical Products (info) | Allocate warehouse inventory to orders                       | Reciprocal | NM   |
| 17 | Physical Products (info) | Analyze supplier quality metrics                             | Pooled     | M    |
| 16 | Physical Products (info) | Develop demand forecasts by product line                     | Pooled     | M    |
| 18 | Physical Products (info) | Plan logistics routes for distribution                       | Pooled     | M    |
| 19 | Physical Products (info) | Schedule production across shared lines                      | Reciprocal | NM   |
| 22 | Service Delivery         | Analyze service quality metrics by region                    | Pooled     | M    |
| 25 | Service Delivery         | Assign service technicians to work orders                    | Reciprocal | NM   |
| 23 | Service Delivery         | Compile service catalog entries                              | Pooled     | M    |
| 21 | Service Delivery         | Document service delivery procedures                         | Pooled     | M    |
| 24 | Service Delivery         | Process service request through fulfillment pipeline         | Sequential | M-O  |
| 26 | Customer Service         | Analyze customer complaint categories                        | Pooled     | M    |
| 30 | Customer Service         | Assign limited warranty replacement inventory                | Reciprocal | NM   |
| 27 | Customer Service         | Draft FAQ and knowledge base articles                        | Pooled     | M    |
| 28 | Customer Service         | Generate customer satisfaction survey reports                | Pooled     | M    |
| 29 | Customer Service         | Triage and route support tickets through escalation pipeline | Sequential | M-O  |
| 35 | Human Capital            | Allocate headcount across departments                        | Reciprocal | NM   |
| 32 | Human Capital            | Compile employee engagement survey analysis                  | Pooled     | M    |
| 31 | Human Capital            | Develop job descriptions for open roles                      | Pooled     | M    |
| 33 | Human Capital            | Develop training curriculum for compliance topics            | Pooled     | M    |
| 34 | Human Capital            | Review and benchmark compensation data                       | Pooled     | M    |
| 36 | Human Capital            | Select candidates from shared applicant pool                 | Reciprocal | NM   |
| 41 | Information Technology   | Allocate cloud compute budget across teams                   | Reciprocal | NM   |
| 37 | Information Technology   | Conduct security vulnerability assessments                   | Pooled     | M    |
| 39 | Information Technology   | Develop software test suites for independent modules         | Pooled     | M    |
| 38 | Information Technology   | Document IT system architecture                              | Pooled     | M    |
| 40 | Information Technology   | Process change request through ITIL pipeline                 | Sequential | M-O  |
| 42 | Information Technology   | Schedule deployment windows on shared environments           | Reciprocal | NM   |
| 48 | Financial Resources      | Allocate capital expenditure across projects                 | Reciprocal | NM   |
| 47 | Financial Resources      | Allocate operating budget across divisions                   | Reciprocal | NM   |
| 44 | Financial Resources      | Analyze expense reports by department                        | Pooled     | M    |
| 49 | Financial Resources      | Assign credit limits from shared credit facility             | Reciprocal | NM   |
| 46 | Financial Resources      | Perform tax compliance analysis by jurisdiction              | Sequential | M-O  |

| #  | APQC Category         | Task                                                 | Thompson   | CALM |
|----|-----------------------|------------------------------------------------------|------------|------|
| 43 | Financial Resources   | Prepare financial statements by entity               | Pooled     | M    |
| 45 | Financial Resources   | Process accounts payable through approval pipeline   | Sequential | M-O  |
| 53 | Assets                | Allocate shared vehicle fleet to departments         | Reciprocal | NM   |
| 51 | Assets                | Analyze asset depreciation schedules                 | Pooled     | M    |
| 50 | Assets                | Conduct asset condition assessments                  | Pooled     | M    |
| 52 | Assets                | Inventory and tag enterprise assets by location      | Pooled     | M    |
| 55 | Risk & Compliance     | Audit regulatory compliance by domain                | Pooled     | M    |
| 54 | Risk & Compliance     | Conduct risk assessments across business functions   | Pooled     | M    |
| 56 | Risk & Compliance     | Develop business continuity plans by department      | Pooled     | M    |
| 57 | Risk & Compliance     | Process regulatory filing through review pipeline    | Sequential | M-O  |
| 61 | External Relations    | Allocate corporate sponsorship budget                | Reciprocal | NM   |
| 60 | External Relations    | Compile ESG disclosures by reporting dimension       | Pooled     | M    |
| 59 | External Relations    | Develop community engagement reports                 | Pooled     | M    |
| 58 | External Relations    | Prepare government affairs briefings by jurisdiction | Pooled     | M    |
| 65 | Business Capabilities | Allocate improvement initiative budget               | Reciprocal | NM   |
| 62 | Business Capabilities | Benchmark operational metrics against industry peers | Pooled     | M    |
| 63 | Business Capabilities | Conduct process maturity assessments                 | Pooled     | M    |
| 64 | Business Capabilities | Evaluate knowledge management practices              | Pooled     | M    |

## 6 SI Text S6. O\*NET Full Results

Table S4 reports monotonicity prevalence by SOC major group with 95% Wilson confidence intervals.

## 7 SI Text S7. LLM Classifier Validation

The 65 APQC tasks were classified by author judgment. To validate that LLMs can replicate this classification (and to support extending it to larger corpora where manual labeling is infeasible), we ran two LLMs (GPT-4.1 mini and Claude Sonnet 4.5) on the same 65 tasks under two prompting conditions, *heuristic* (the five-test decision table from Table S1) and *raw* (definitions only, no heuristics). The heuristic prompt provides the task description and the five-test decision table (Table S1); the raw prompt provides the task description and the definitions of monotone and non-monotone specifications without the heuristic tests. Full prompt text is available in the code repository. Each condition was run 3 times at temperature 0. Author labels serve as ground truth.

Following Eloundou et al. [17], who used GPT-4 to annotate  $\sim 19,000$  O\*NET task statements for LLM exposure, we treat LLM annotation as a scalable proxy for expert judgment when validated

Table S4: O\*NET monotonicity prevalence by SOC major group. M = coordination-free, M-O = requires ordering only, NM = requires coordination. 95% Wilson CIs.

| SOC Major Group                                | M           | M-O        | NM          | % Mono     | 95% CI          |
|------------------------------------------------|-------------|------------|-------------|------------|-----------------|
| Life, Physical, and Social Science             | 404         | 83         | 442         | 52%        | [49, 56]        |
| Sales and Related                              | 131         | 14         | 143         | 50%        | [45, 56]        |
| Community and Social Service                   | 99          | 9          | 108         | 50%        | [43, 57]        |
| Healthcare Support                             | 111         | 20         | 142         | 48%        | [42, 54]        |
| Personal Care and Service                      | 158         | 31         | 216         | 47%        | [42, 52]        |
| Office and Administrative Support              | 219         | 57         | 353         | 44%        | [40, 48]        |
| Healthcare Practitioners and Technical         | 504         | 95         | 767         | 44%        | [41, 46]        |
| Business and Financial Operations              | 248         | 38         | 377         | 43%        | [39, 47]        |
| Protective Service                             | 166         | 7          | 235         | 42%        | [38, 47]        |
| Building and Grounds Cleaning and Maintenance  | 44          | 5          | 68          | 42%        | [33, 51]        |
| Farming, Fishing, and Forestry                 | 46          | 8          | 75          | 42%        | [34, 50]        |
| Production                                     | 413         | 137        | 775         | 42%        | [39, 44]        |
| Arts, Design, Entertainment, Sports, and Media | 178         | 34         | 313         | 40%        | [36, 45]        |
| Transportation and Material Moving             | 201         | 23         | 332         | 40%        | [36, 44]        |
| Food Preparation and Serving Related           | 94          | 12         | 158         | 40%        | [34, 46]        |
| Construction and Extraction                    | 256         | 98         | 528         | 40%        | [37, 43]        |
| Computer and Mathematical                      | 177         | 47         | 341         | 40%        | [36, 44]        |
| Installation, Maintenance, and Repair          | 216         | 79         | 475         | 38%        | [35, 42]        |
| Architecture and Engineering                   | 273         | 79         | 575         | 38%        | [35, 41]        |
| Educational Instruction and Library            | 396         | 50         | 794         | 36%        | [33, 39]        |
| Legal                                          | 24          | 4          | 56          | 33%        | [24, 44]        |
| Management                                     | 243         | 33         | 579         | 32%        | [29, 35]        |
| <b>Total</b>                                   | <b>4601</b> | <b>963</b> | <b>7852</b> | <b>41%</b> | <b>[41, 42]</b> |

against a hand-labeled sample.

All four configurations achieve  $\geq 95\%$  accuracy and  $\kappa \geq 0.88$  (Table S5). The error pattern is consistent across models. Every misclassification labels a monotonic task as non-monotonic (false non-monotonic), never the reverse. This bias is safe, as it over-coordinates rather than under-coordinates.

## 8 SI Text S8. Simulation Protocol

**Tasks.** Ten tasks from the corpus span the monotonicity spectrum (Table S6). We decompose each task into 3–5 specialist agents, fixing sub-task descriptions and validity criteria before execution.

**Coordinated condition.** An orchestrator LLM (GPT-4.1 mini, temperature 0) manages the full execution pipeline. It first receives the task description and plans sub-task assignments. It then formats and delivers each assignment to the corresponding agent. Agents execute in order; for sequential tasks, the orchestrator passes prior-stage output to each downstream agent. After all agents complete, the orchestrator reviews the collected outputs for consistency. For non-monotonic tasks, it reconciles conflicting requests to produce a final allocation within the shared constraints. The coordinated token totals in Table S7 include all tokens consumed by orchestrator planning, formatting, and review calls.

Table S5: Classification accuracy of LLM-based monotonicity classifiers on the 65-task corpus. Metrics computed on 2-class labels (M+M-O vs. NM) from Run 1. Self-consistency measured across 3 runs.

| Model             | Condition | Mono F1 | NM F1 | Macro F1 | $\kappa$ | Consistency |
|-------------------|-----------|---------|-------|----------|----------|-------------|
| GPT-4.1 mini      | Heuristic | 0.968   | 0.919 | 0.943    | 0.887    | 61/65       |
| GPT-4.1 mini      | Raw       | 0.989   | 0.971 | 0.980    | 0.961    | 64/65       |
| Claude Sonnet 4.5 | Heuristic | 0.989   | 0.971 | 0.980    | 0.961    | 64/65       |
| Claude Sonnet 4.5 | Raw       | 0.968   | 0.919 | 0.943    | 0.887    | 62/65       |

**Uncoordinated condition.** Each agent receives only its sub-task description, with no orchestrator intermediary. For the sequential task, we still pass prior-stage output to the next agent as causal delivery. No orchestrator reviews, reconciles, or reformats outputs. We concatenate agent outputs sequentially under labeled section headers.

**Validity evaluation.** GPT-4.1 mini acts as LLM-as-judge, running separately from the experiment agents. The evaluator receives the task-specific validity prompt plus the full final output and reasons step-by-step against each criterion before writing VALID or INVALID on the final line. We track evaluation tokens separately and exclude them from the coordinated and uncoordinated token totals.

**Token overhead ratios.** Table S7 reports the coordinated/uncoordinated token ratio for each task and model. These are the empirical  $c$  values used in the Coordination Tax.

## 9 SI Text S9. Sensitivity Analysis

### 9.1 Reclassification Range

The 74% prevalence figure holds at APQC Levels 2–3 (team-level workflows). Reclassifying all borderline cases yields 60–74% monotonic. The lower bound (60%) assumes every borderline task is non-monotonic; the upper bound (74%) is the observed rate. Coarser decomposition pushes toward non-monotonic because bundling tasks together increases the chance of introducing shared constraints. Finer decomposition pushes toward monotonic because smaller sub-tasks are more likely to be independent.

### 9.2 Decomposition Dependence

The prevalence figure reflects the task decompositions we chose, not only the tasks themselves. A task that is monotonic under one sub-task assignment may become non-monotonic under another. For example, a report-writing task is monotonic if sections are independent but becomes non-monotonic if two sections share a word count budget. More broadly, the Bridge Theorem and Coordination Tax apply to any multi-agent setting where tasks can be decomposed and classified, but the prevalence parameter depends on the unit of analysis. APQC’s 74% reflects team-level workflows that decompose naturally into multi-agent sub-tasks. O\*NET’s 42% reflects individual work activities that may or may not warrant multi-agent treatment. Software engineering, scientific research, and creative workflows would yield different distributions still (code review, for instance, is inherently reciprocal).

### 9.3 Hidden Constraints

The most dangerous failure mode is a task that appears monotonic but carries implicit non-monotonic constraints (e.g., unstated consistency requirements across independent reports). The reverse also occurs. Tasks that look non-monotonic may decompose into monotonic sub-tasks if resources are pre-partitioned.

## References

- [1] Tom J. Ameloot, Frank Neven, and Jan Van den Bussche. Relational transducers for declarative networking. *Journal of the ACM*, 60(2):1–38, 2013.
- [2] Joseph M. Hellerstein. The coordination criterion. *arXiv preprint arXiv:2602.09435*, 2026.
- [3] Leslie Lamport. Time, clocks, and the ordering of events in a distributed system. *Communications of the ACM*, 21(7):558–565, 1978.
- [4] Joseph M. Hellerstein and Peter Alvaro. Keeping CALM: When distributed consistency is easy. *Communications of the ACM*, 63(9):72–81, 2020.
- [5] Marc Shapiro, Nuno Preguiça, Carlos Baquero, and Marek Zawirski. Conflict-free replicated data types. In *Stabilization, Safety, and Security of Distributed Systems (SSS)*, pages 386–400. Springer, 2011.
- [6] Jay R. Galbraith. Organization design: An information processing view. *Interfaces*, 4(3):28–36, 1974.
- [7] Henry Mintzberg. *The Structuring of Organizations*. Prentice-Hall, Englewood Cliffs, NJ, 1979.
- [8] Herbert A. Simon. The architecture of complexity. *Proceedings of the American Philosophical Society*, 106(6):467–482, 1962.
- [9] Lyra J. Colfer and Carliss Y. Baldwin. The mirroring hypothesis: Theory, evidence, and exceptions. *Industrial and Corporate Change*, 25(5):709–738, 2016.
- [10] Ronald H. Coase. The nature of the firm. *Economica*, 4(16):386–405, 1937.
- [11] Oliver E. Williamson. *The Economic Institutions of Capitalism*. Free Press, New York, 1985.
- [12] William G. Ouchi. Markets, bureaucracies, and clans. *Administrative Science Quarterly*, 25(1):129–141, 1980.
- [13] Ivan D. Steiner. *Group Process and Productivity*. Academic Press, New York, 1972.
- [14] Jaeho Lee and Christos A. Makridis. Task-level automation and workers’ skills in the age of AI. *Information Economics and Policy*, 64:101054, 2023.
- [15] Thomas W. Malone and Kevin Crowston. The interdisciplinary study of coordination. *ACM Computing Surveys*, 26(1):87–119, 1994.
- [16] Peter Bailis, Alan Fekete, Michael J. Franklin, Ali Ghodsi, Joseph M. Hellerstein, and Ion Stoica. Coordination avoidance in database systems. *Proceedings of the VLDB Endowment*, 8(3):185–196, 2015.

- [17] Tyna Eloundou, Sam Manning, Pamela Mishkin, and Daniel Rock. GPTs are GPTs: Labor market impact potential of LLMs. *Science*, 384(6702):1306–1308, 2024.

Table S6: Tasks used in the simulations with pre-specified validity criteria.

| Task              | Type             | Agents | Validity criterion                                                                                                                                                          |
|-------------------|------------------|--------|-----------------------------------------------------------------------------------------------------------------------------------------------------------------------------|
| Strategy pillars  | Pooled (M)       | 4      | All four pillars present (Market Expansion, Technology Investment, Operational Excellence, Talent Development), each with a strategic objective and at least one initiative |
| Feature specs     | Pooled (M)       | 4      | All four module specs present (Authentication, Search, Reporting, Notifications), each with scope, API endpoints, and data model                                            |
| Marketing content | Pooled (M)       | 4      | Content present for all four channels (email, social media, blog, press release), each with headline, body, and CTA; no contradictions on product name or value proposition |
| Security audit    | Pooled (M)       | 4      | All four layer reports present (Network, Application, Data, Identity), each with at least one finding with severity rating and recommendation                               |
| Stage-gate review | Sequential (M-O) | 3      | All three stages present (technical, market, financial); market references technical findings; financial references both; no factual contradictions                         |
| Ticket escalation | Sequential (M-O) | 3      | All three tiers present (L1 Triage, L2 Resolution, L3 Specialist); L2 references L1 categories; L3 references L2 resolution attempt; no contradictions                      |
| Budget alloc.     | Reciprocal (NM)  | 5      | All five divisions represented; total allocation $\leq \$50,000,000$                                                                                                        |
| Backlog sprint    | Reciprocal (NM)  | 4      | Features from all four domains represented (UX, Backend, Infrastructure, Integrations); total story points $\leq 200$                                                       |
| Production sched. | Reciprocal (NM)  | 4      | All four products scheduled (Alpha, Beta, Gamma, Delta); Line 1 $\leq 40$ hrs; Line 2 $\leq 40$ hrs                                                                         |
| Headcount alloc.  | Reciprocal (NM)  | 5      | All five departments have allocations (Engineering, Sales, Customer Success, Marketing, Operations); total $\leq 25$ positions                                              |

Table S7: Simulation results: Coordinated/uncoordinated token ratio ( $c$ ) by task and model (10 runs per condition, temperature 0). These are the empirical  $c$  values used in the Coordination Ceiling (Equation 1).

| Task              | Type | GPT-4.1-mini | Haiku 4.5   | Sonnet 4.5  |
|-------------------|------|--------------|-------------|-------------|
| Strategy pillars  | M    | $3.1\times$  | $2.7\times$ | $2.9\times$ |
| Feature specs     | M    | $2.5\times$  | $2.7\times$ | $2.6\times$ |
| Marketing content | M    | $3.3\times$  | $4.0\times$ | $3.9\times$ |
| Security audit    | M    | $3.2\times$  | $2.7\times$ | $2.6\times$ |
| Stage-gate        | M-O  | $2.3\times$  | $2.7\times$ | $2.7\times$ |
| Ticket escalation | M-O  | $2.9\times$  | $3.0\times$ | $2.8\times$ |
| Budget alloc.     | NM   | $3.6\times$  | $3.2\times$ | $3.4\times$ |
| Backlog sprint    | NM   | $3.5\times$  | $3.4\times$ | $3.4\times$ |
| Production sched. | NM   | $4.4\times$  | $4.3\times$ | $4.2\times$ |
| Headcount alloc.  | NM   | $2.9\times$  | $3.1\times$ | $3.0\times$ |
